# Supplementary material for: Probabilistic Soundness Guarantees in LLM Reasoning Chains
Source: arXiv:2507.12948 source file (2025-09-28)
Supplement: Supplementary file 1 [file 06-related-dump.tex]

\section{Detailed Related Works}

\paragraph{Evaluating CoT.}
ROSCOE~\citep{golovneva2023roscoe} propose a suite of metrics for scoring step-by-step reasoning using alignment of a step with the most similar previous step using a trained similarity model using contrastive learning.
ReCEval~\citep{prasad-etal-2023-receval} evaluates the correctness of a step using intra-step correctness and inter-step correctness using entailment model and Pointwise V-Information.
SocREal~\citep{he2024socrevallargelanguagemodels} prompt LLM to automatically evaluate based on Socratic method.
